# Supplementary material for: Emergent fractals in dirty topological crystals
Source: arXiv:2504.17786 ancillary file (2025-11-12)
Supplement: Supplementary file 1 [file Supplementary_EmergentFractal.pdf]

# Supplemental Material:
# Emergent fractals in dirty topological crystals

Daniel J. Salib[1] and Bitan Roy[1]

[1] *Department of Physics, Lehigh University, Bethlehem, Pennsylvania, 18015, USA*

(Dated: April 24, 2025)

Supplemental Material contains details of the (a) kernel polynomial method to compute the projector ($\mathcal{P}$) [Sec. S1] and (b) computation of the fractal and anomalous dimensions [Sec. S2].

## S1. DETAILS OF THE KERNEL POLYNOMIAL METHOD (KPM)

In this section, we discuss the details of the KPM employed to compute the projector ($\mathcal{P}$) in disordered Chern insulators, which we use to compute the disorder-averaged Bott index $\langle B \rangle$. In KPM, a function is expanded as a series of Chebyshev polynomials. The Chebyshev polynomials of the first and second kind are two related series of polynomials of a variable $x$ which are mutually orthogonal under the inner product defined over the real interval $x \in [-1, 1]$ and a certain respective weight function [1]. We consider only the Chebyshev polynomials of the first kind $T_n(x)$ which have the weight function $w(x) = (\pi\sqrt{1-x^2})^{-1}$. This definition yields the orthogonality relation

$$\langle T_n | T_m \rangle = \int_{-1}^{1} \frac{T_n(x) T_m(x)}{\pi\sqrt{1-x^2}}\, dx = \frac{1+\delta_{n,0}}{2} \delta_{n,m}. \tag{S1}$$

Although a closed-form expression exists for the polynomial of degree $n$, given by $T_n(x) = \cos(n \arccos(x))$, this form is not computationally feasible for matrix-valued polynomials. An equivalent and more tractable construction is given by the iterative series

$$T_0(x) = 1, \quad T_1(x) = x, \quad \text{and} \quad T_n(x) = 2x T_{n-1}(x) - T_{n-2}(x) \quad \text{for} \quad n \geq 2. \tag{S2}$$

Because of their orthogonality, computational efficiency, and simplicity (compared to other orthogonal polynomials), the Chebyshev polynomials form an ideal and numerically stable basis for expanding a given one-dimensional function $f(x)$, where $-1 \leq x \leq 1$. This expansion takes the form

$$f(x) = \sum_{n=0}^{\infty} a_n T_n(x), \tag{S3}$$

where the moments $a_n$ are given by

$$a_n = \frac{\langle f | T_n \rangle}{\langle T_n | T_n \rangle} = \frac{2}{1+\delta_{n,0}} \int_{-1}^{1} \frac{f(x) T_n(x)}{\pi\sqrt{1-x^2}}\, dx. \tag{S4}$$

More generally, an operator $A$ which depends on another operator $\Lambda$ and some variable parameter $\nu$ has the expansion

$$A(\nu, \Lambda) = \sum_{n=0}^{\infty} a_n(\nu) T_n(\Lambda), \text{where} \quad a_n(\nu) = \frac{2}{1+\delta_{n,0}} \int_{-1}^{1} \frac{A(\nu, \lambda) T_n(\lambda)}{\pi\sqrt{1-\lambda^2}}\, d\lambda, \tag{S5}$$

where $\lambda \in [-1, 1]$ is the spectrum of $\Lambda$ [2].

### A. Gibbs oscillations and the Jackson kernel

Obviously, as with any series expansion, the Chebyshev series may only be carried out to some arbitrary finite order for numerical computation. However, a trivial truncation of Eq. (S5) often leads to numerical instability near regions where the spectrum of $\Lambda$ is not smooth, especially around discontinuities and singularities [1]. This manifests as fluctuations in the quantity being evaluated, which is known as the Gibbs oscillations. A well-established method for mitigating Gibbs oscillations is to introduce convolution of the evaluated operator with an aptly chosen kernel

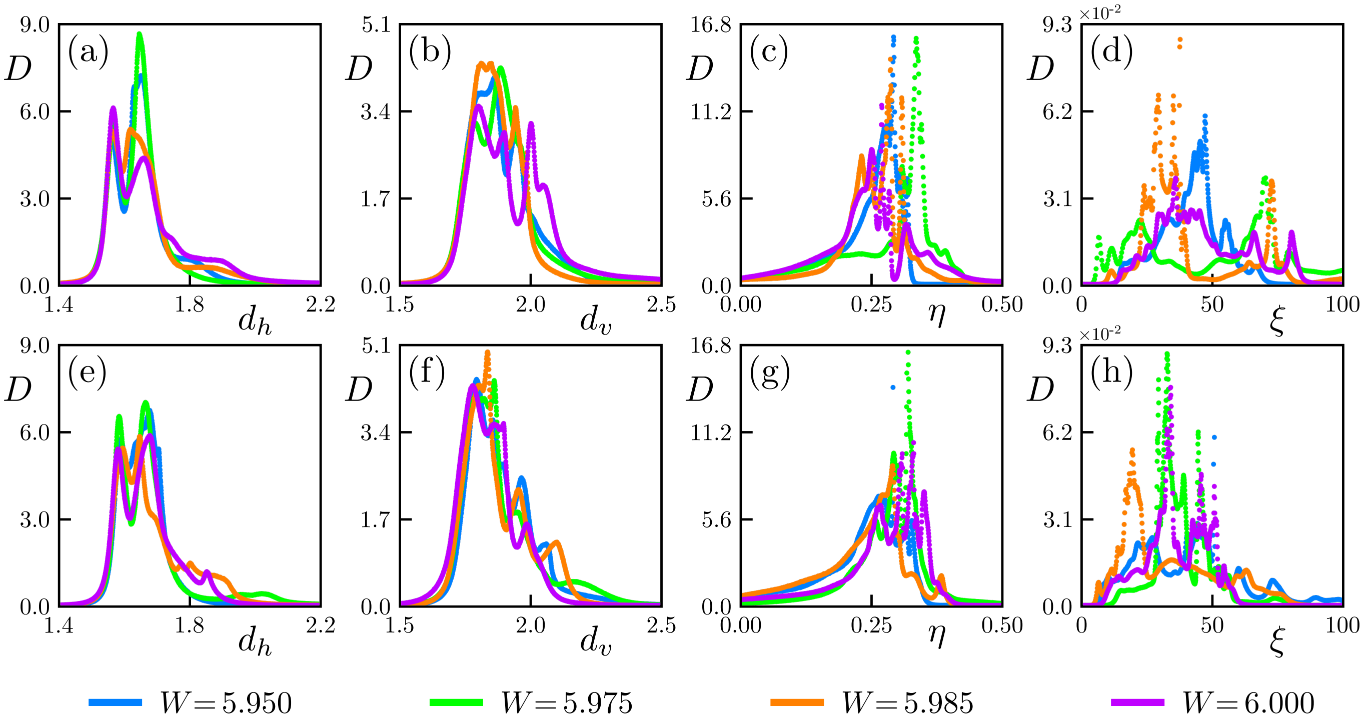


Figure S1. Distributions of the various fractal characteristics of interest as computed during Bayesian bootstrap analyses. Each curve corresponds to the relative frequency of yielding a given value during sampling. Columns (a)-(d) respectively display the distributions of the hull fractal dimension $d_h$, volume fractal dimension $d_v$, anomalous dimension $\eta$, and correlation length $\xi$ of trivial fractal clusters. Columns (e)-(h) are analogous, but corresponding to topological clusters. Data are color coded according to disorder strength (see legend), and all results are obtained after averaging over various system sizes (see Sec.S2).

when performing the Chebyshev expansion. This procedure effectively modifies the moments by introducing a new coefficient in each term which depends on the particular kernel and the truncation order $N$.

In general, these coefficients may also depend on additional kernel-dependent parameters, but henceforth we consider only the Jackson kernel which takes no specified parameters besides $N$. The Jackson kernel is among the most commonly used kernels for its versatility and is ideal for most applications. Without showing the explicit form of this kernel, one finds that the convolution process results in the Jackson coefficients

$$g_n^{\mathrm{Jac}} = \frac{1}{N+1}\left[(N-n+1)\cos\left(\frac{\pi n}{N+1}\right) + \sin\left(\frac{\pi n}{N+1}\right)\cot\left(\frac{\pi}{N+1}\right)\right]. \tag{S6}$$

Implementation of the kernel method is straightforward: truncate Eq. (S5) at order $N$ and make the replacement $a_n(\nu) \to g_n^{\mathrm{Jac}} a_n(\nu)$.

### B. Application of KPM for computing the projector

In the-zero temperature limit, the action of the projector ($\mathcal{P}$) onto the states below the Fermi energy can be approximated by a KPM expansion of the Heaviside step function [2]

$$\mathcal{P}(E_F, H) = \Theta(E_F - H) \approx \sum_{n=0}^{N} g_n^{\mathrm{Jac}} b_n(\tilde{E_F}) T_n(\tilde{H}). \tag{S7}$$

Here, $\tilde{H}$ is a necessary shifting and scaling of the original Hamiltonian to ensure that the spectrum is constrained to the interval $[-1,1]$. Then, $\tilde{E}_F$ is the corresponding shifted and scaled Fermi energy. Explicitly, we have

$$\begin{gathered}\tilde{H} = (H-b)/a, \ \ \text{and} \ \ \tilde{E}_F = (E_F - b)/a, \\ \text{where} \ \ a \equiv (E_{\max} - E_{\min})/(2-\epsilon), \ \ \text{and} \ \ b \equiv (E_{\max} + E_{\min})/2.\end{gathered} \tag{S8}$$

The parameter $\epsilon$ is a small buffer (set to be 0.01 in all presented computations) which ensures that the spectrum of $\tilde{H}$ is constrained to $[-1+\epsilon, 1-\epsilon]$. Exclusion of the end points $-1$ and 1 is necessary as truncating the operator expansion to finite order generally leads to numerical instability at these points.

Finally, a closed-form expression for the moments $b_n(\tilde{E_F})$ can be found by evaluating the integral in Eq.(S5) for the Heaviside step function, given by

$$b_n(\tilde{E_F}) = \begin{cases} 1 - \frac{\arccos(\tilde{E_F})}{\pi} & n = 0 \\ -\frac{2\sin[n \arccos(\tilde{E_F})]}{n\pi} & n > 0 \end{cases}. \tag{S9}$$

Computation of the Bott index then follows as usual once the projector ($\mathcal{P}$) is constructed, which we show in the main manuscript in detail. We compute $\mathcal{P}$ with 2048 KPM moments.

## S2. DETAILS OF THE FRACTAL ANALYSIS

In this section, we discuss details related to the analysis of emergent fractals close to the topological insulator (TI) to normal insulator (NI) quantum phase transition (QPT). Analyzing distinct fractal clusters in small systems proves challenging for various reasons. The fractal clusters emerge across a range of size scales but share self-similar structure. However, there exists a lower limit on the cluster size below which they lack the complexity to exhibit defining fractal characteristics. Small systems may not have sufficient space to accommodate a significant number of clusters, even at the smallest size scale. Additionally, they lack the capacity to host clusters over a wide range of larger size scales. This issue is exacerbated by the necessity to trim the local Chern marker (LCM) distribution at the edges to remove numerical anomalies induced by finite-size effects. Consequently, due to computational costs associated with simulating sufficiently large systems, our analysis is limited to a few strengths of disorder in the vicinity of the disorder-induced TI-NI quantum critical point (QCP), located at $W \approx 6.0$, where $W$ denotes the disorder strength. In all computations pertaining to the following discussion, we consider system of $L = 60, 80, 100$, and 120 for the computation of the fractal dimensions $d_h$ and $d_v$, and $L = 80, 100$, and 120 for the computation of the pair connectivity from which we extract the anomalous dimension $\eta$ and the correlation length $\xi$. Here, $L$ denotes the linear dimension of the square lattice in each direction. In our analysis, we compute these quantities independently from the fractal clusters of TIs and NIs. The results are summarized in Figure S1.

The raw data entering our analysis consists of LCM distributions obtained for multiple disorder realizations of a lattice system at various disorder strengths around the critical point. Each LCM distribution is initially continuous-valued, reflecting spatial fluctuations in the underlying topology. Prior to extracting fractal clusters, it is necessary to discretize these distributions. To ensure a robust discretization and minimize the influence of isolated numerical fluctuations, we first apply a Gaussian convolution to smooth each LCM distribution according to

$$\tilde{\mathcal{C}}(\mathbf{r}_i) = \text{round}\left[\sum_{\Delta} K(\Delta)\, \mathcal{C}_{\text{loc}}(\mathbf{r}_i + \Delta)\right], \tag{S10}$$

where the sum runs over displacements $\Delta$ to the nearest and next-nearest-neighbor sites of $i$, and $K(\Delta)$ is a Gaussian kernel with standard deviation $\sigma = 0.5$. The convoluted values are then rounded, and all sites of a given value that are mutually connected through nearest neighbor proximity are classified under the same fractal cluster. Examples are shown in Figs. 1(h) and 1(i) of the main manuscript. Then within each such cluster, we compute the radius of gyration ($R$), the perimeter ($P$), the area ($A$), and the pair connectivity ($G$), following the prescription mentioned in the main manuscript. Subsequently, we extract the hull fractal dimension ($d_h$), the volume fractal dimension ($d_v$), the anomalous dimension ($\eta$), and the correlation length ($\xi$). Results are shown in Fig. 2 of the main manuscript.

### A. Weighted Bayesian Bootstrapping

As mentioned, larger clusters are more favorable due to their higher-quality features, in contrast to smaller clusters that may be too small to exhibit self-similar features on a discrete lattice. This issue is exacerbated by the characteristic skew of the cluster size distribution toward smaller clusters. To ensure more equal representation across size scales, stochastic weighting is used to resample the data using a method known as Bayesian bootstrapping. This approach

assigns statistical weights to clusters in data-space-based manner, balancing the representation of cluster sizes and pair connectivity scales effectively. Specifically, each cluster is assigned a probability weight that is the product of two factors:

1. **Density compensation factor:** Geometric properties of each cluster (primarily radius $R$ and area $A$) are first approximated by a multivariate kernel density estimate (KDE) constructed over the combined $R$–$A$ space of all clusters. Clusters situated in densely populated regions of this parameter space receive smaller weights, whereas those in sparser regions are weighted more heavily. This step ensures uniform statistical representation of cluster sizes, mitigating biases towards overly abundant small-scale clusters. Similar weight compensation is applied when fitting pair connectivity distances.

2. **Bayesian window prior:** For each bootstrap iteration, we generate a random distribution of sampling weights defined by a superposition of Gaussian windows whose parameters (center, width, and amplitude) are themselves randomly sampled from predetermined statistical distributions. Specifically, the full data range is first partitioned into a specified number of bins. A Gaussian window is assigned to each bin, and the amplitude of this window as well as its central position and width relative to the bin are randomly varied. The entire range is considered at each iteration, but the varying positions, widths, and amplitudes of these Gaussian windows create diverse sampling profiles. This random hierarchical sampling approach effectively explores all possible weighting partitions of the data, extensively accounting for inherent data uncertainty, numerical instabilities, and arbitrariness in fitting procedures.

Additionally, we systematically varied several other analysis parameters, including whether to perform fits directly or using a log-log fit, the inclusion or exclusion of density compensation, the choice of minimum cluster size used in the analysis ($A_{\rm min}$), and the maximum distance cutoff ($r_{\rm max}$) considered when fitting the pair connectivity function. A comprehensive parameter sweep was performed over all these variations, ensuring robustness and strong validation of the statistical rigor of our extracted fractal dimensions and correlation parameters.

All data were fitted according to the corresponding prescriptions mentioned in the main manuscript, and 2000 samples were taken for each individual set of bootstrap variations. The hull fractal dimension ($d_h$), volume fractal dimension ($d_v$), anomalous dimension ($\eta$), and correlation length ($\xi$) values were compiled across all iterations into respective comprehensive distributions. The means and standard deviations of these distributions were taken to represent the reported values within error.

### B. Pair Connectivity Computation

Finally, a comment is due regarding the computation of $G(r)$. Since each cluster contributes independently to the pair connectivity, $G(r)$ can alternatively be expressed as a mean over the ensemble of all clusters labeled by $\mu$

$$G(r) = \langle G(r \mid \mu) \rangle_{\mu} . \tag{S11}$$

This formulation allows for a more tractable numerical evaluation of the pair connectivity, reducing the problem to computing each $G(r \mid \mu)$. To proceed, we first precompute two arrays $r^{\rm global}$ and $\Delta^{\rm global}$. The first one-dimensional array stores

$$r^{\rm global} = \left[ r_0^{\rm global}, r_1^{\rm global}, ..., r_{N_r-1}^{\rm global} \right] = \left[ 1, \sqrt{2}, ..., \sqrt{2}L \right] , \tag{S12}$$

which stores all unique possible distances between any two sites in an $L \times L$ lattice, sorted in order, with a total of $N_r$ unique distance values; and a two-dimensional array $\Delta^{\rm global}$ of shape $(L^2, N_r)$. We use $n_r$ as a simple index $(0 \leq n_r < N_r)$ that steps through the ordered list of distinct non-zero lattice separations $r_{n_r}^{\rm global}$. To construct $r^{\rm global}$ we calculate the distances between every pair of sites $i$ and $j$ on the lattice, where $i, j \in [1, L^2]$ and $i \neq j$, defined as

$$R_{i,j} = \sqrt{(x_i - x_j)^2 + (y_i - y_j)^2}. \tag{S13}$$

Extracting the unique non-zero distances and sorting them produces $r^{\rm global}$. The second array $\Delta^{\rm global}$ is initialized to zeros and is used to store the counts of these distances for each site. To populate $\Delta^{\rm global}$, we count, for each site $i$, how many sites $j$ correspond to each unique distance $r_{n_r}^{\rm global}$ and store this count in $\Delta_{i,n_r}^{\rm global}$. In other words, $\Delta_{i,n_r}^{\rm global}$

represents the number of lattice sites that are exactly at a distance $r_{n_r}^{\text{global}}$ away from site $i$.

With these arrays prepared, we now compute $G(r \mid \mu)$ for a given cluster $\mu$, which consists of a subset of occupied sites $\{i\} \subset [1, L^2]$. To calculate $G(r \mid \mu)$, we determine the distances between all pairs of occupied sites $i \neq j$ within the cluster and count how many pairs correspond to each unique distance $r_{n_r}^{\text{global}}$. These counts are stored in $\Delta^{\mu}$, where $\Delta_{n_r}^{\mu}$ represents the number of pairs within the cluster separated by $r_{n_r}^{\text{global}}$. To normalize these counts, we use the precomputed global counts $\Delta^{\text{global}}$. Summing $\Delta_{i,n_r}^{\text{global}}$ over all occupied sites $i$ in the cluster gives $\Delta_{n_r}^{\text{cluster}}$, which is the total number of possible pairs at each distance within the cluster. The pair connectivity for the cluster is then given by

$$G(r_{n_r}^{\text{global}} \mid \mu) = \frac{\Delta_{n_r}^{\mu}}{\Delta_{n_r}^{\text{cluster}}}. \tag{S14}$$

Averaging $G(r \mid \mu)$ over all clusters yields the overall pair connectivity $G(r)$ for the lattice.

[1] A. Weiße, G. Wellein, A. Alvermann, and H. Fehske, The kernel polynomial method, Rev. Mod. Phys. **78**, 275 (2006).
[2] D. Varjas, M. Fruchart, A. R. Akhmerov, and P. M. Perez-Piskunow, Computation of topological phase diagram of disordered $Pb_{1-x}Sn_xTe$ using the kernel polynomial method, Phys. Rev. Res. **2**, 013229 (2020).
